# Supplementary material for: The Beatbots: A Musician-Informed Multi-Robot Percussion Quartet
Source: arXiv:2502.00966 source file (2025-02-03)
Supplement: Supplementary file 1 [file appendix.tex]

\newpage
\appendix

\section*{Figure and Table Descriptions} \label{descrip}
Don't look here yet. I didn't write this. Oops.

Table \ref{tab:survey-codes}: TODO
